# Supplementary material for: Slow Thermalization Between a Lattice and Free Bose Gas
Source: arXiv:1211.4772 ancillary file (2013-07-27)
Supplement: Supplementary file 1 [file spindeplattice_therm_supp_v2.pdf]

# Supplemental Material for “Slow Thermalization Between a Lattice and Free Bose Gas”

David C. McKay,<sup>1,\*</sup> Carolyn Meldgin,<sup>1</sup> David Chen,<sup>1</sup> and Brian DeMarco<sup>1</sup>

*<sup>1</sup>Department of Physics, University of Illinois,  
1110 W Green St., Urbana, IL 61801*

(Dated: July 26, 2013)

## EXPERIMENTAL PARAMETERS

The two spin components are separated during time-of-flight using a magnetic field gradient. For the measurement shown in Fig. 2, we use  $75 \times 10^3$   $|1\rangle$  atoms and  $20 \times 10^3$   $|0\rangle$  atoms and a  $\nu = (44.5 \pm 0.6)$  Hz (geometric mean) trap frequency. We used  $(14 \pm 3) \times 10^3$   $|0\rangle$  and  $(45 \pm 7) \times 10^3$   $|1\rangle$  atoms and  $\nu = (75 \pm 6)$  Hz for the measurements in Fig. 3 and 4. We calibrate the lattice potential depth  $s$  using Kapitza-Dirac diffraction of a BEC in the  $|1\rangle$  state. Averaging the FGR calculations shown in Fig. 4 over the  $|1\rangle$  density profile does not significantly alter those results.

## SPATIAL OVERLAP BETWEEN SPECIES

We perform two measurements to rule out lack of spatial overlap as an explanation for suppression of inter-species thermalization. The  $|1\rangle$  and  $|0\rangle$  atoms can separate for two reasons. Since the  $|1\rangle$  and  $|0\rangle$  states have different magnetic moments, stray magnetic-field gradients can separate the two gases. Interactions may also cause the mixture to phase separate. For a co-trapped condensates in a harmonic trap, the stability condition against phase separation is [1]

$$a_{10}^2 < a_{11}a_{00}, \quad (1)$$

where  $a_{xy}$  is the scattering length for a binary collision between atoms in state  $x$  and  $y$ . The scattering lengths in our mixture are  $a_{11} = (100.4 \pm 0.1)a_0$ ,  $a_{00} = (100.9 \pm 0.1)a_0$ , and  $a_{10} = (100.4 \pm 0.1)a_0$  [2], so the stability criterion is satisfied ( $a_0$  is the Bohr radius). As we explain in the discussion that follows, we do not observe any evidence for phase separation.

We check for spatial segregation on long and short length scales using two separate methods. Spatial separation on long length scales (i.e., greater than a few  $\mu\text{m}$ ) is probed using in-situ images of the different components. Fits to these images are used to determine the center of each component. The inter-species separation (in the imaging plane) between centers is plotted in Fig. 1 for two cases: separately prepared gases and a mixture. Within the  $3 \mu\text{m}$  imaging resolution of our imaging system, there is no significant separation between the centers of the gases. Furthermore, there is no significant difference whether we prepare the two components separately or in a mixture. The data in Fig. 1 are therefore consistent with spatial overlap between the two species on length scales greater than approximately 10

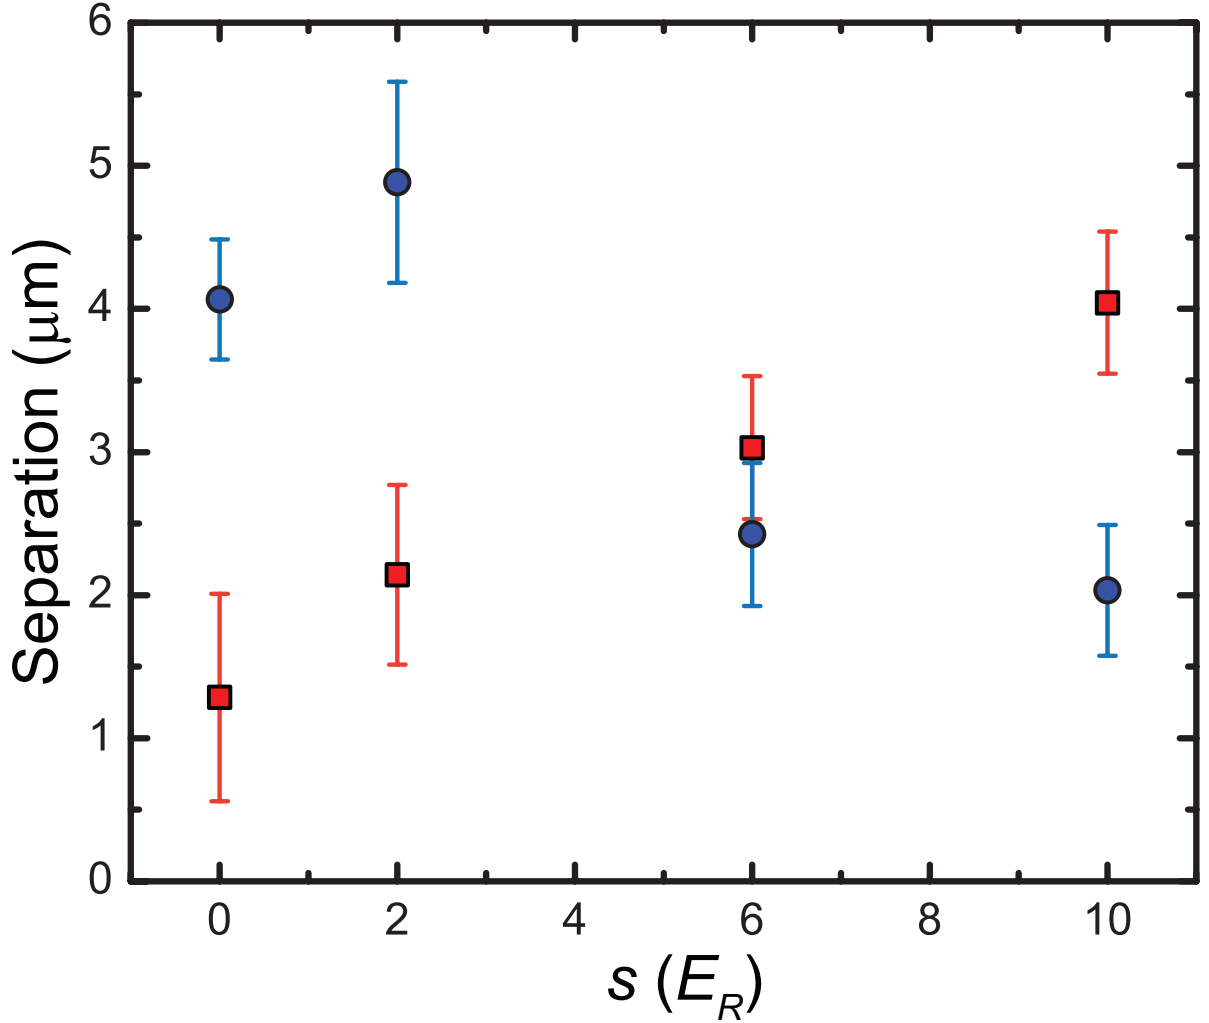

FIG. 1. In-situ separation between the centers of the  $|0\rangle$  and  $|1\rangle$  gases as a function of the lattice depth when the two gases are prepared in the same trap (blue circles) and when the gases are prepared separately in subsequent experimental runs (red squares). The FWHM of the gases is approximately  $15\text{--}20\ \mu\text{m}$ . The error bars are the standard error of the mean from averaging over 4 experimental runs.

lattice spacings.

On the lattice length scale, it is possible that the  $|0\rangle$  atoms are repelled (through inter-species interactions) by the  $|1\rangle$  atoms from the minima of the lattice potential. Since the resolution of our imaging system is approximately  $3\ \mu\text{m}$  and the lattice spacing is  $0.4\ \mu\text{m}$ , we cannot directly detect this type of microscopic phase separation. Therefore, we employ a microwave spectroscopy technique that has lattice-length-scale resolution averaged over

the trap. We use pulses of a microwave-frequency magnetic field to transfer atoms from the  $|0\rangle$  state to the  $|F=2, m_F=1\rangle$  state, which is trapped in the same lattice potential as the  $|1\rangle$  atoms (the spin-dependent lattice potential depth is only a function of  $g_F m_F$ , which is the same for these two states, where  $g_F$  is the gyromagnetic ratio). An  $80\ \mu\text{s}$  pulse (sufficiently long to resolve the lattice bands) is employed, and we drive the  $|0\rangle$  atoms directly to the lowest energy  $|2, 1\rangle$  lattice band. The Rabi rate  $\Omega$  for this process is proportional to the overlap  $\langle\psi_0(\vec{x})|w(\vec{x})\rangle$  of the  $|0\rangle$  atomic wavefunctions  $\psi(\vec{x})$  with the Wannier-state wavefunctions  $w(\vec{x})$  for the lattice (which coincide with the positions of the  $|1\rangle$  atoms) [3].

To demonstrate this effect, we transfer a gas composed of only  $|0\rangle$  atoms to the  $|2, 1\rangle$  state with and without the lattice present. Figure 2 shows that the fraction transferred on resonance is reduced when the lattice is present. A fit of the data in Fig. 2 to a Rabi lineshape indicates that the ratio of Rabi rates is  $0.42 \pm 0.07$ , in approximate agreement with the prediction  $\Omega \propto \langle\psi_0(\vec{x})|w(\vec{x})\rangle \approx 0.57$ , where we treat  $\psi_0(\vec{x})$  as spatially uniform on the lattice length scale.

With a mixture of  $|0\rangle$  and  $|1\rangle$  atoms present, a decrease in the number of  $|0\rangle$  atoms transferred to the  $|2, 1\rangle$  state is an indication that microscopic phase separation has occurred. In Fig. 3 we show the results of this test. For a fixed duration microwave pulse, the number of atoms transferred to the  $|2, 1\rangle$  state is constant, whether or not  $|1\rangle$  atoms are present. Thus, there is clear evidence for spatial overlap between the  $|0\rangle$  and  $|1\rangle$  atoms on the lattice length scale.

## DEPHASING

Here we describe the dephasing procedure in more detail, and we provide data demonstrating that dephasing leaves the density distribution largely unaffected. For dephasing, the lattice is ramped up to  $s = 19$  and down to  $s = 4$  in  $100\ \mu\text{s}$  to prevent transitions to higher bands. A series of three pulses (Fig. 4) is used to prevent phase revivals [4]. The time-of-flight images in Fig. 4 of the  $|1\rangle$  atoms before and after the dephasing procedure show that an approximately uniform quasimomentum distribution  $n_q$  is generated, which is equivalent to the  $\tilde{T} \rightarrow \infty$  limit. The slight modulation in  $n_q$  at  $s = 4$  corresponds to a temperature more than an order of magnitude greater than that of the  $|0\rangle$  component. These images are taken after turning off the lattice suddenly (in  $10\ \text{ns}$ ) and  $20\ \text{ms}$  TOF.

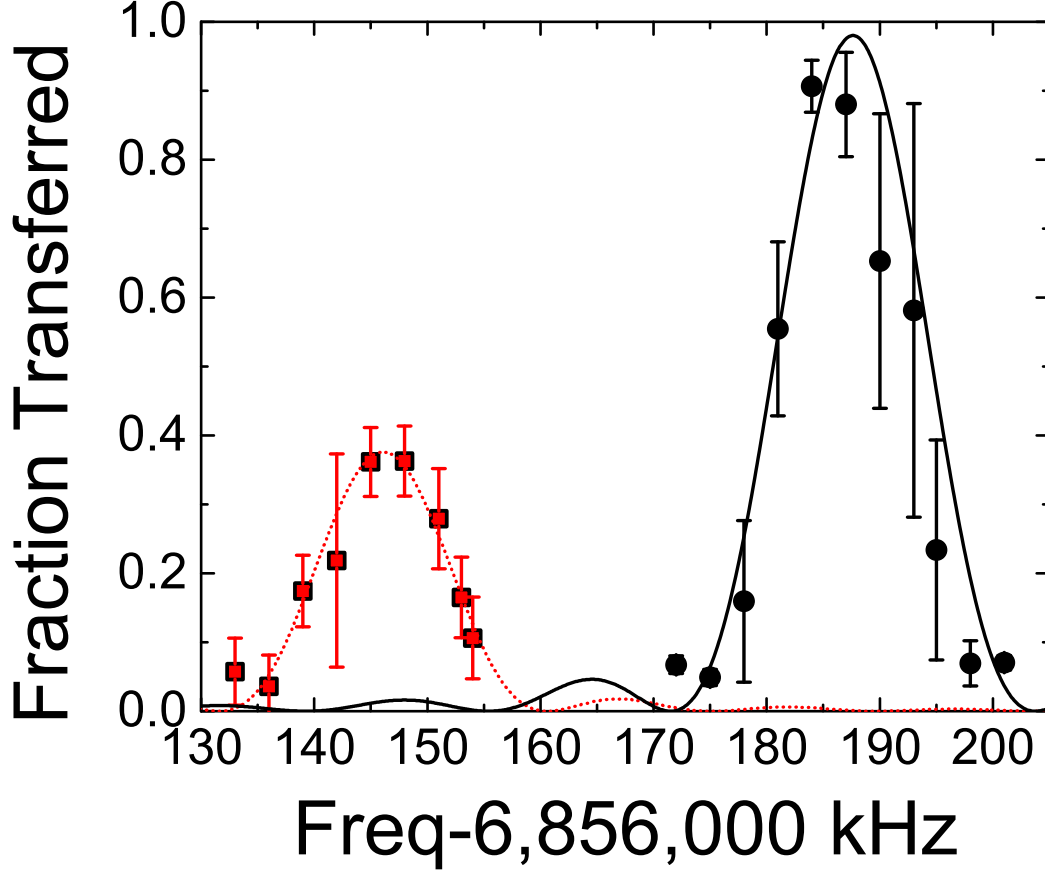

FIG. 2. Transferring atoms from the  $|0\rangle$  to the  $|2, 1\rangle$  state using a  $80 \mu\text{s}$  duration microwave pulse. We measure the fraction of atoms transferred as the microwave frequency is varied. Atoms are transferred without a lattice (black circles) and when a lattice with potential depth  $s = 12$  for the  $|2, 1\rangle$  atoms is present. The lines are a fit to a Rabi lineshape for the data with (dotted red line) and without (solid black line) a lattice present. The shift in central frequency arises because of the lattice band structure. The error bars in this and the next figure show the standard error in the mean for the average across experimental runs.

The quasimomentum distribution  $n_q$  along a lattice direction perpendicular to the imaging direction is shown as a slice through the image. The quasimomentum  $q$  corresponding to each imaged position is computed according to the lattice wavevector and the TOF. The imaged slice is restricted to positions equivalent to momentum within the first Brillouin zone, where  $q_B$  is the momentum at the edge of the Brillouin zone.

In interpreting the data shown in Fig. 4 in the main text, we assume that the dephasing

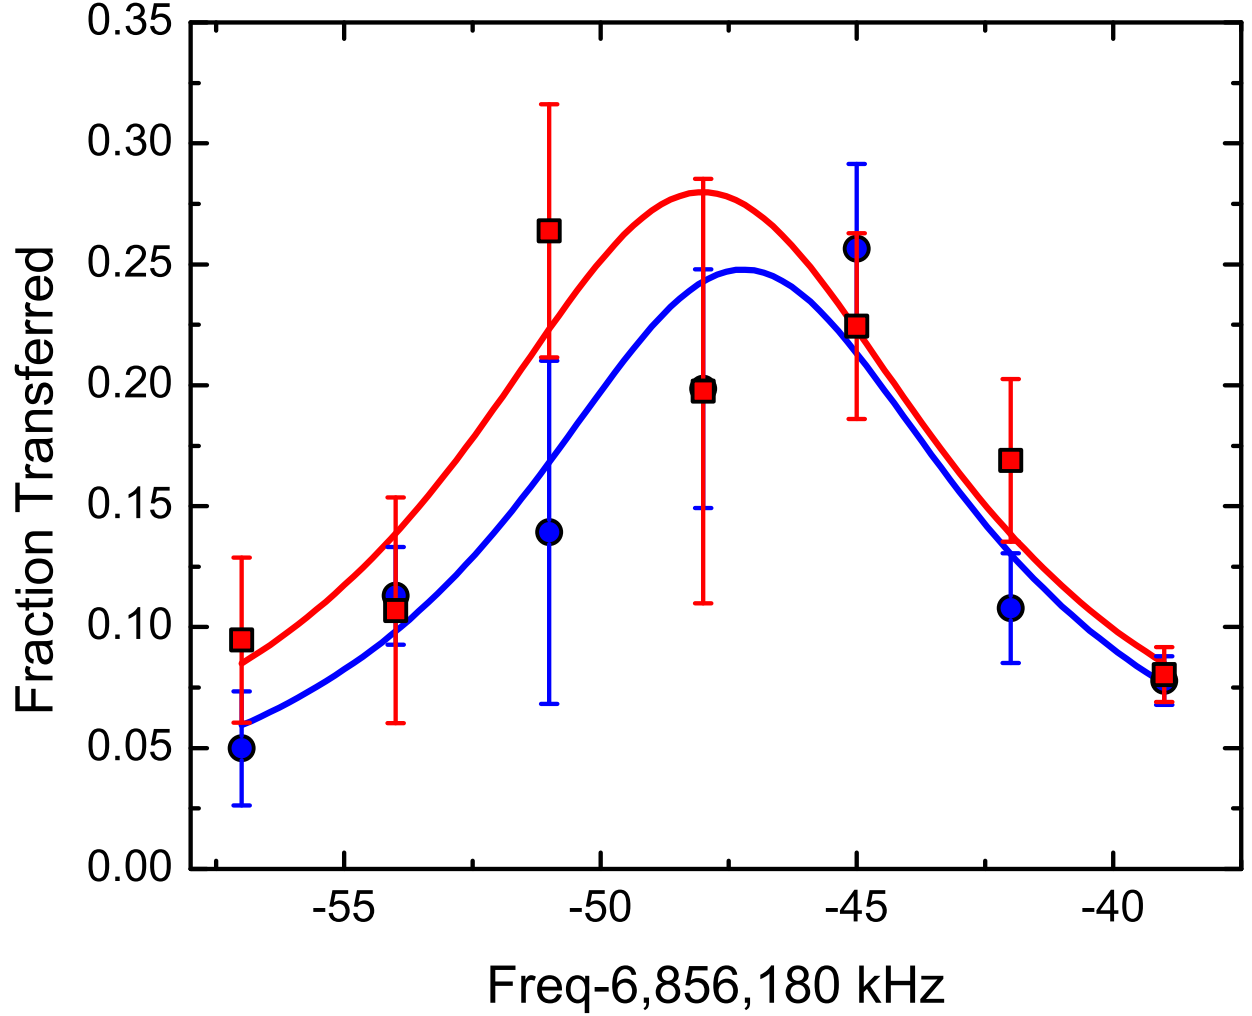

FIG. 3. Atoms are transformed from the  $|0\rangle$  to the  $|2, 1\rangle$  state with and without  $|1\rangle$  atoms present. There are approximately  $1.5 \times 10^4$  atoms in the  $|0\rangle$  state, and for the data with a mixture there are also  $(5.3 \pm 0.6) \times 10^4$   $|1\rangle$  atoms. Data taken with only  $|0\rangle$  atoms are shown using red squares, and with a mixture using blue circles. The lines are Lorentzian fits to the data. Within the fit uncertainty, the fraction of atoms transferred is unaffected by the presence of  $|1\rangle$  atoms, demonstrating that microscopic phase separation does not occur. Interaction effects on these frequency scales are small; at  $s = 12$ ,  $U = h \times 1.26$  kHz.

procedure does not change the  $|1\rangle$  density distribution. We characterize density redistribution using in-situ images to determine the size of the gas via a fit to a Gaussian distribution. Data are shown in Fig. 5 with and without the dephasing procedure. As expected, minor density distribution occurs at lower lattice depths where the tunneling rate is higher. Be-

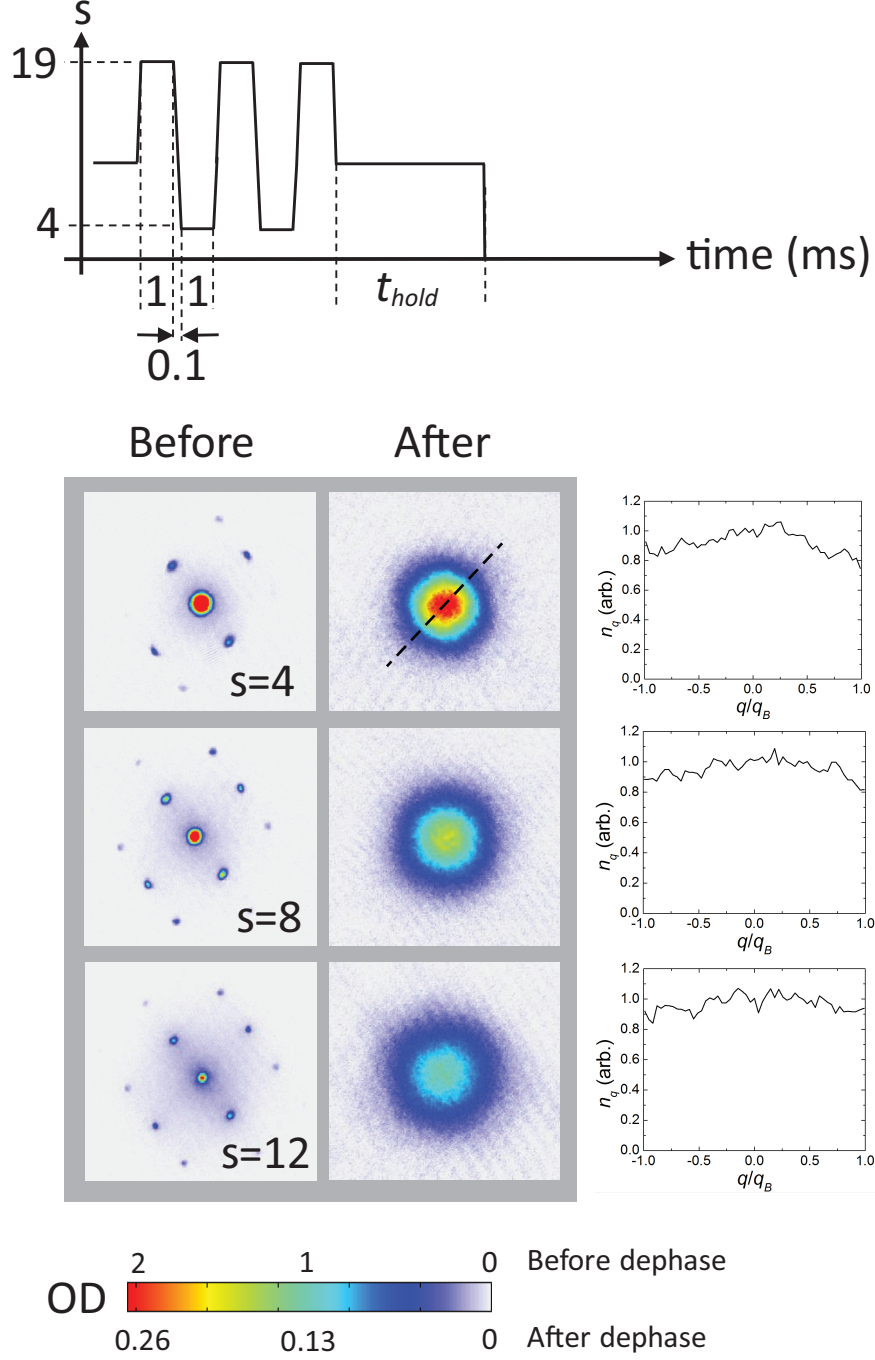

FIG. 4. Dephasing procedure (top) and images of the lattice ( $|1\rangle$ ) gas before and after the dephasing procedure. The color scale indicates the measured optical depth. Slices through the imaged density profile along a lattice direction (indicated by the dashed line) are shown. Each image is the average over five experimental iterations, and each quasimomentum distribution is averaged over five adjacent slices.

cause we assume that the  $|1\rangle$  density is fixed in our FGR calculation, the suppression of inter-species thermalization may be an even larger effect than is evident in Fig. 4 in the main text.

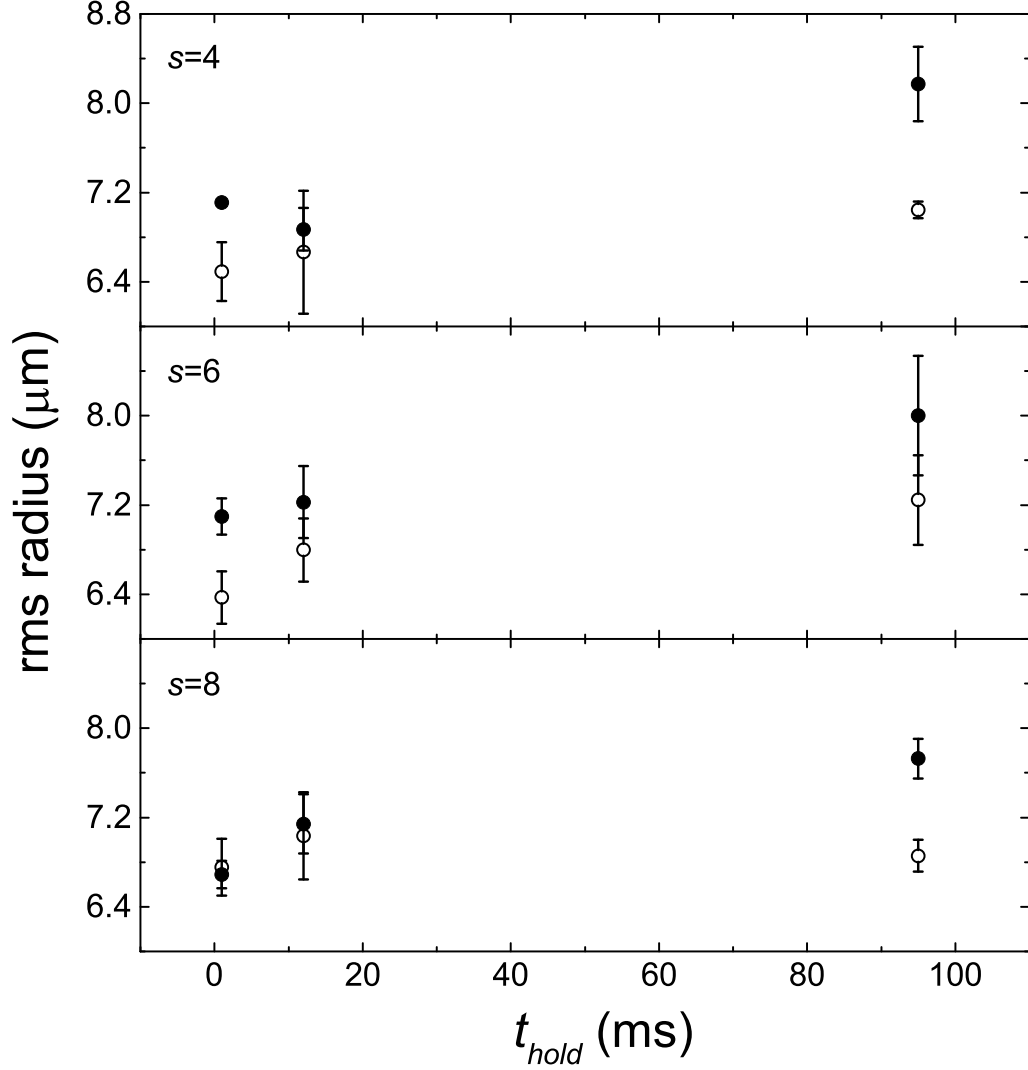

FIG. 5. Radius of the lattice gas with (solid circles) and without (open circles) the dephasing procedure at  $s = 4, 6, 8$ . At  $t_{\text{hold}} = 0$  ms (i.e., immediately after the dephasing procedure), there is less than a 10% change in the rms radius of the gas. More of the energy added by dephasing is transferred to the spatial degrees of freedom after  $t_{\text{hold}} = 95$  ms. This effect decreases at higher lattice depths where the tunneling time is longer. The assumption of constant  $|1\rangle$  density is excellent for the measurement of  $\dot{T}$ , given that  $t_{\text{hold}} \leq 12$  ms for those data. This assumption is worse at lower lattice depths, and leads to underestimating the thermalization rate. The error bars are the standard deviation for an average over 3 experimental runs.

---

\* Now at:James Franck Institute, 929 E 57th Street, Chicago, IL 60637

- [1] C. J. Pethick and H. Smith, *Bose-Einstein condensation in dilute gases* (Cambridge University Press, 2002).
- [2] E. G. M. van Kempen, S. J. J. M. F. Kokkelmans, D. J. Heinzen, and B. J. Verhaar, Phys. Rev. Lett. **88**, 093201 (2002).
- [3] L. Förster, M. Karski, J.-M. Choi, A. Steffen, W. Alt, D. Meschede, A. Widera, E. Montano, J. H. Lee, W. Rakreungdet, and P. S. Jessen, Phys. Rev. Lett. **103**, 233001 (2009).
- [4] M. Greiner, O. Mandel, T. W. Hänsch, and I. Bloch, Nature **419**, 51 (2002).
